# Supplementary material for: AMaRaNTA: Automated First-Principles Exchange Parameters In 2D Magnets
Source: arXiv:2509.20226 ancillary file (2025-09-24)
Supplement: Supplementary file 1 [file AMaRaNTA_SUPPL_MAT.pdf]

## SUPPLEMENTARY MATERIAL

In Table S1, we provide the 12 parameters (exchange plus SIA) that are directly output of AMaRaNTA, without any further processing.

| Material                          | $J_{xx}^{(1)}$ | $J_{yy}^{(1)}$ | $J_{zz}^{(1)}$ | $J_{xy}^{(1)}$ | $J_{yx}^{(1)}$ | $J_{xz}^{(1)}$ | $J_{zx}^{(1)}$ | $J_{yz}^{(1)}$ | $J_{zy}^{(1)}$ | $J^{(2)}$ | $J^{(3)}$ | $A$   |
|-----------------------------------|----------------|----------------|----------------|----------------|----------------|----------------|----------------|----------------|----------------|-----------|-----------|-------|
| CrBrO                             | -1.56          | -1.56          | -1.57          | 0.00           | 0.00           | -0.01          | -0.01          | 0.00           | 0.00           | -0.78     | -8.05     | -0.03 |
| CrBrS                             | -6.53          | -6.48          | -6.56          | 0.00           | -0.00          | 0.26           | -0.27          | 0.02           | 0.02           | -9.74     | -9.31     | -0.02 |
| CrBr <sub>3</sub>                 | -3.34          | -3.28          | -3.36          | 0.05           | 0.05           | -0.03          | -0.03          | -0.05          | -0.05          | -0.43     | 0.23      | -0.04 |
| CrClO                             | -1.58          | -1.56          | -1.58          | -0.00          | -0.00          | -0.01          | -0.01          | 0.01           | 0.00           | -0.80     | -7.44     | -0.07 |
| CrCl <sub>3</sub>                 | -2.58          | -2.57          | -2.58          | -0.00          | 0.00           | 0.01           | 0.01           | -0.00          | -0.00          | -0.23     | 0.21      | -0.01 |
| CrGeTe <sub>3</sub>               | -11.96         | -11.52         | -12.21         | -0.30          | -0.30          | -0.04          | -0.04          | 0.04           | 0.04           | 0.16      | -1.13     | 0.09  |
| CrI <sub>3</sub>                  | -3.15          | -4.22          | -3.83          | 0.00           | -0.00          | 0.48           | 0.48           | 0.00           | 0.00           | -0.81     | 0.18      | -0.10 |
| CrPS <sub>4</sub>                 | -9.86          | -9.86          | -9.86          | -0.01          | -0.01          | -0.02          | -0.02          | -0.01          | -0.01          | -9.01     | -0.48     | -0.03 |
| CrSiSe <sub>3</sub>               | 5.13           | 5.18           | 5.11           | -0.04          | -0.04          | 0.01           | 0.01           | -0.02          | -0.02          | 0.08      | 1.85      | 0.02  |
| CrSiTe <sub>3</sub>               | -10.30         | -11.16         | -11.10         | 0.01           | 0.01           | 0.12           | 0.12           | -0.00          | 0.00           | -0.13     | -0.83     | 0.10  |
| MnO <sub>2</sub>                  | -3.13          | -3.12          | -3.12          | -0.02          | -0.02          | 0.03           | 0.03           | 0.02           | 0.02           | -0.35     | 2.19      | -0.21 |
| MnBi <sub>2</sub> Te <sub>4</sub> | -0.21          | -0.29          | -0.12          | 0.02           | 0.02           | -0.00          | -0.00          | 0.02           | 0.02           | 0.32      | 0.22      | -0.18 |
| MnBr <sub>2</sub>                 | 1.12           | 1.12           | 1.11           | 0.01           | 0.01           | 0.00           | 0.00           | 0.00           | 0.00           | 0.16      | 0.45      | -0.02 |
| MnCl <sub>2</sub>                 | 1.20           | 1.19           | 1.19           | 0.01           | 0.01           | -0.00          | -0.00          | 0.00           | 0.00           | 1.80      | 0.07      | -0.00 |
| MnI <sub>2</sub>                  | 0.91           | 0.93           | 0.90           | 0.02           | 0.02           | -0.01          | -0.01          | -0.01          | -0.01          | 0.34      | 0.68      | -0.01 |
| NiBr <sub>2</sub>                 | -4.41          | -4.51          | -4.48          | 0.08           | 0.08           | 0.11           | 0.11           | 0.06           | 0.06           | -0.05     | 3.33      | 0.02  |
| NiCl <sub>2</sub>                 | -4.80          | -4.79          | -4.79          | -0.00          | -0.00          | -0.01          | -0.01          | -0.00          | -0.00          | -0.06     | 1.89      | 0.00  |
| NiI <sub>2</sub>                  | -3.39          | -4.62          | -4.60          | 1.13           | 1.13           | 1.31           | 1.31           | 0.69           | 0.69           | -0.30     | 7.10      | 0.28  |
| NiO <sub>8</sub> Re <sub>2</sub>  | -1.26          | -1.26          | -1.28          | -0.00          | -0.00          | -0.01          | -0.01          | -0.00          | -0.01          | 0.01      | 0.03      | -0.22 |
| NiF <sub>4</sub> Tl <sub>2</sub>  | 22.02          | 22.02          | 22.00          | 0.04           | 0.04           | 0.00           | -0.00          | -0.00          | -0.00          | 0.39      | 0.34      | -0.02 |
| NiPS <sub>3</sub>                 | -4.10          | -4.10          | -4.12          | -0.00          | -0.00          | -0.00          | -0.00          | -0.00          | -0.00          | 1.05      | 29.49     | 0.05  |
| NiPSe <sub>3</sub>                | -3.69          | -3.73          | -3.80          | 0.03           | 0.03           | -0.04          | -0.04          | 0.07           | 0.07           | -0.63     | 32.67     | -0.12 |
| VAgP <sub>2</sub> Se <sub>6</sub> | -1.93          | -1.93          | -1.94          | -0.27          | 0.26           | -0.07          | 0.06           | -0.17          | 0.17           | 0.10      | 0.07      | -0.04 |
| VCl <sub>2</sub>                  | 7.01           | 7.01           | 7.01           | -0.00          | -0.00          | 0.00           | 0.00           | 0.00           | 0.00           | 0.13      | 0.27      | -0.03 |
| VBr <sub>2</sub> O                | 4.48           | 4.48           | 4.48           | 0.00           | -0.00          | -0.00          | -0.00          | 0.00           | 0.00           | -0.14     | -8.52     | 0.07  |
| VBr <sub>2</sub>                  | 12.26          | 12.26          | 12.27          | -0.01          | -0.01          | 0.01           | 0.01           | -0.01          | -0.01          | 7.78      | 0.17      | -0.01 |
| VF <sub>4</sub>                   | 6.09           | 6.08           | 6.07           | 0.02           | -0.02          | 0.30           | -0.30          | -0.22          | 0.22           | 0.13      | 0.25      | -0.08 |
| VI <sub>2</sub>                   | 3.98           | 4.02           | 4.01           | -0.04          | -0.04          | 0.04           | 0.04           | -0.07          | -0.07          | 1.06      | 0.15      | -0.02 |
| VPS <sub>3</sub>                  | 96.20          | 96.19          | 96.20          | 0.01           | 0.01           | 0.01           | 0.01           | 0.01           | 0.01           | 5.90      | 5.51      | -0.03 |

TABLE S1. Exchange parameters and SIA, in meV, as directly produced by AMaRaNTA.

In the following, we provide quantities not directly produced by AMaRaNTA, yet easily obtained by simple post-processing of the code's direct output. Table S2 shows the decomposition of the nearest-neighbour exchange tensor into the matrices  $\underline{\mathbf{K}}_{ij}$  and  $\underline{\mathbf{D}}_{ij}$ , as introduced in the Results section of the main document (only the independent matrix elements are reported).

| Material                          | $K_{xx}$ | $K_{yy}$ | $K_{zz}$ | $K_{xy}$ | $K_{xz}$ | $K_{yz}$ | $D_{xy}$ | $D_{xz}$ | $D_{yz}$ |
|-----------------------------------|----------|----------|----------|----------|----------|----------|----------|----------|----------|
| CrBrO                             | 0.00     | 0.00     | -0.01    | 0.00     | -0.01    | 0.00     | 0.00     | 0.00     | 0.00     |
| CrBrS                             | -0.01    | 0.05     | -0.04    | -0.04    | 0.00     | -0.00    | 0.02     | 0.26     | -0.00    |
| CrBr <sub>3</sub>                 | -0.01    | 0.05     | -0.03    | -0.03    | 0.05     | -0.03    | -0.05    | -0.00    | 0.00     |
| CrClO                             | -0.00    | 0.01     | -0.01    | -0.01    | 0.01     | 0.01     | 0.00     | 0.00     | 0.00     |
| CrCl <sub>3</sub>                 | -0.00    | 0.01     | -0.00    | -0.00    | 0.00     | 0.01     | -0.00    | -0.00    | -0.00    |
| CrGeTe <sub>3</sub>               | -0.07    | 0.38     | -0.31    | -0.30    | 0.04     | 0.04     | -0.00    | 0.00     | 0.00     |
| CrI <sub>3</sub>                  | -0.10    | 0.59     | -0.49    | -0.10    | 0.48     | 0.00     | 0.00     | 0.00     | 0.00     |
| CrPS <sub>4</sub>                 | -0.00    | 0.00     | -0.00    | -0.00    | -0.02    | -0.01    | -0.01    | -0.01    | 0.00     |
| CrSiSe <sub>3</sub>               | -0.01    | 0.04     | -0.03    | -0.04    | 0.01     | -0.02    | 0.00     | 0.00     | 0.00     |
| CrSiTe <sub>3</sub>               | 0.56     | -0.31    | -0.25    | 0.01     | 0.12     | 0.00     | 0.00     | 0.00     | 0.00     |
| MnO <sub>2</sub>                  | -0.01    | 0.01     | -0.00    | -0.02    | 0.03     | 0.02     | 0.00     | -0.00    | -0.00    |
| MnBi <sub>2</sub> Te <sub>4</sub> | -0.00    | -0.09    | 0.09     | 0.02     | -0.00    | 0.02     | -0.00    | -0.00    | -0.00    |
| MnBr <sub>2</sub>                 | 0.00     | 0.00     | -0.00    | 0.00     | 0.00     | 0.00     | 0.00     | 0.00     | 0.00     |
| MnCl <sub>2</sub>                 | 0.00     | 0.00     | -0.00    | 0.00     | 0.00     | 0.00     | 0.00     | 0.00     | 0.00     |
| MnI <sub>2</sub>                  | -0.00    | 0.02     | -0.02    | 0.02     | -0.01    | -0.01    | -0.00    | -0.01    | 0.00     |
| NiBr <sub>2</sub>                 | 0.05     | -0.04    | -0.01    | 0.08     | 0.11     | 0.06     | 0.00     | -0.00    | 0.00     |
| NiCl <sub>2</sub>                 | -0.00    | 0.00     | -0.00    | -0.00    | -0.00    | -0.00    | 0.00     | 0.00     | 0.00     |
| NiI <sub>2</sub>                  | 0.28     | 0.82     | -0.42    | -0.40    | 1.13     | 1.31     | 0.69     | 0.00     | 0.01     |
| NiO <sub>8</sub> Re <sub>2</sub>  | 0.01     | 0.01     | -0.02    | 0.01     | -0.00    | -0.01    | 0.00     | 0.00     | 0.00     |
| NiF <sub>4</sub> Tl <sub>2</sub>  | 0.00     | -0.01    | -0.01    | 0.00     | 0.04     | -0.00    | -0.00    | 0.00     | 0.01     |
| NiPS <sub>3</sub>                 | 0.01     | 0.00     | -0.01    | 0.00     | -0.00    | -0.00    | -0.00    | 0.00     | 0.00     |
| NiPSe <sub>3</sub>                | 0.05     | 0.01     | -0.06    | 0.03     | -0.00    | 0.03     | 0.07     | -0.00    | -0.00    |
| VAgP <sub>2</sub> Se <sub>6</sub> | -0.00    | -0.01    | -0.01    | -0.01    | -0.27    | -0.06    | 0.06     | -0.17    | 0.17     |
| V1Cl <sub>2</sub>                 | -0.00    | 0.00     | -0.00    | -0.00    | 0.00     | 0.00     | 0.00     | 0.00     | 0.00     |
| VBr <sub>2</sub> O                | 0.00     | -0.00    | -0.00    | -0.00    | -0.00    | 0.00     | 0.00     | 0.00     | 0.00     |
| VBr <sub>2</sub>                  | -0.01    | -0.00    | 0.00     | 0.00     | -0.01    | -0.01    | 0.00     | 0.00     | 0.00     |
| VF <sub>4</sub>                   | 0.02     | -0.00    | -0.01    | -0.00    | 0.30     | -0.22    | 0.02     | 0.30     | -0.22    |
| VI <sub>2</sub>                   | -0.04    | 0.02     | 0.01     | 0.01     | 0.04     | -0.07    | -0.04    | 0.04     | -0.07    |
| VPS <sub>3</sub>                  | 0.00     | 0.00     | 0.00     | 0.00     | 0.01     | 0.01     | 0.01     | 0.01     | 0.01     |

TABLE S2. Decomposition of the nearest-neighbour exchange tensor into the matrices  $\underline{\mathbf{K}}_{ij}$  and  $\underline{\mathbf{D}}_{ij}$  [meV].

Finally, in Table S3, we list some other useful quantities obtained after post-processing and discussed in the main document.

| Material                          | $J^{(1)}$ | $\max(\underline{\mathbf{K}})/J^{(1)}$ | $\text{avg}(\underline{\mathbf{K}})/J^{(1)}$ | $D$  | $\arctan(D/J^{(1)})$ | $J^{(2)}/J^{(1)}$ | $J^{(3)}/J^{(1)}$ |
|-----------------------------------|-----------|----------------------------------------|----------------------------------------------|------|----------------------|-------------------|-------------------|
| CrBrO                             | -1.57     | 0.00                                   | 0.00                                         | 0.00 | 0.00                 | 0.50              | 5.14              |
| CrBrS                             | -6.52     | 0.01                                   | 0.00                                         | 0.26 | 0.04                 | 1.49              | 1.43              |
| CrBr <sub>3</sub>                 | -3.33     | 0.02                                   | 0.01                                         | 0.00 | 0.00                 | 0.13              | -0.07             |
| CrClO                             | -1.57     | 0.01                                   | 0.00                                         | 0.00 | 0.00                 | 0.50              | 4.72              |
| CrCl <sub>3</sub>                 | -2.57     | 0.00                                   | 0.00                                         | 0.00 | 0.00                 | 0.09              | -0.08             |
| CrGeTe <sub>3</sub>               | -11.90    | 0.03                                   | 0.02                                         | 0.00 | 0.00                 | -0.01             | 0.09              |
| CrI <sub>3</sub>                  | -3.73     | 0.16                                   | 0.07                                         | 0.00 | 0.00                 | 0.22              | 0.10              |
| CrPS <sub>4</sub>                 | -9.86     | 0.00                                   | 0.00                                         | 0.00 | 0.00                 | 0.91              | 0.05              |
| CrSiSe <sub>3</sub>               | 5.14      | 0.01                                   | 0.01                                         | 0.00 | 0.00                 | 0.02              | 0.36              |
| CrSiTe <sub>3</sub>               | -10.85    | 0.05                                   | 0.02                                         | 0.00 | 0.00                 | 0.01              | 0.08              |
| MnO <sub>2</sub>                  | -3.12     | 0.01                                   | 0.00                                         | 0.00 | 0.00                 | 0.11              | 0.70              |
| MnBi <sub>2</sub> Te <sub>4</sub> | -0.21     | 0.43                                   | 0.18                                         | 0.00 | 0.00                 | -1.53             | -1.08             |
| MnBr <sub>2</sub>                 | 1.12      | 0.01                                   | 0.00                                         | 0.00 | 0.00                 | 0.15              | 0.40              |
| MnCl <sub>2</sub>                 | 1.19      | 0.01                                   | 0.00                                         | 0.00 | 0.00                 | 1.50              | 0.06              |
| MnI <sub>2</sub>                  | 0.91      | 0.02                                   | 0.01                                         | 0.00 | 0.00                 | 0.37              | 0.74              |
| NiBr <sub>2</sub>                 | -4.47     | 0.02                                   | 0.01                                         | 0.00 | 0.00                 | 0.01              | -0.74             |
| NiCl <sub>2</sub>                 | -4.79     | 0.00                                   | 0.00                                         | 0.00 | 0.00                 | 0.01              | -0.39             |
| NiI <sub>2</sub>                  | -4.20     | 0.31                                   | 0.19                                         | 0.00 | 0.00                 | 0.07              | -1.69             |
| NiO <sub>8</sub> Re <sub>2</sub>  | -1.27     | 0.01                                   | 0.01                                         | 0.00 | 0.00                 | -0.01             | -0.02             |
| NiF <sub>4</sub> Tl <sub>2</sub>  | 22.01     | 0.00                                   | 0.00                                         | 0.00 | 0.00                 | 0.02              | 0.02              |
| NiPS <sub>3</sub>                 | -4.10     | 0.00                                   | 0.00                                         | 0.00 | 0.00                 | -0.26             | -7.19             |
| NiPSe <sub>3</sub>                | -3.74     | 0.02                                   | 0.01                                         | 0.00 | 0.00                 | -0.17             | -8.73             |
| VAgP <sub>2</sub> Se <sub>6</sub> | -1.94     | 0.00                                   | 0.00                                         | 0.32 | 0.17                 | -0.05             | -0.04             |
| VCl <sub>2</sub>                  | 7.01      | 0.00                                   | 0.00                                         | 0.00 | 0.00                 | 0.02              | 0.04              |
| VBr <sub>2</sub> O                | 4.48      | 0.00                                   | 0.00                                         | 0.00 | 0.00                 | -0.03             | -1.90             |
| VBr <sub>2</sub>                  | 12.27     | 0.00                                   | 0.00                                         | 0.00 | 0.00                 | 0.63              | 0.01              |
| VF <sub>4</sub>                   | 6.08      | 0.00                                   | 0.00                                         | 0.37 | 0.06                 | 0.02              | 0.04              |
| VI <sub>2</sub>                   | 4.00      | 0.02                                   | 0.01                                         | 0.00 | 0.00                 | 0.26              | 0.04              |
| VPS <sub>3</sub>                  | 96.20     | 0.00                                   | 0.00                                         | 0.00 | 0.00                 | 0.06              | 0.06              |

TABLE S3. Remaining post-processing quantities: isotropic nearest-neighbour scalar parameter  $J^{(1)}$  [meV], ratios  $\max(\underline{\mathbf{K}})/J^{(1)}$  and  $\text{avg}(\underline{\mathbf{K}})/J^{(1)}$  (discussed in Fig. 3 of the main text), length of the Dzyaloshinskii–Moriya vector  $D$  [meV] and angle  $\arctan(D/J^{(1)})$  (discussed in Fig. 4 of the main text), ratios  $J^{(2)}/J^{(1)}$  and  $J^{(3)}/J^{(1)}$ .
